# Supplementary material for: GroPrompt: Efficient Grounded Prompting and Adaptation for Referring Video Object Segmentation
Source: arXiv:2406.12834 source file (2024-06-23)
Supplement: Supplementary file 1 [file supp.tex]

\clearpage
\setcounter{page}{1}

\maketitlesupplementary

\section{More Experimental Results}
% \subsection{Ablation Studies}

% To verify the effectiveness of our proposed loss functions, we conduct ablation studies by taking the ground-truth bounding boxes to compute the IoU scores of the predicted box proposals on Ref-DAVIS17. From Table~\ref{tab:ablation}, we see that when only $L_{box}$ is considered, the box and segmentation score \( \mathcal{J} \)\&\( \mathcal{F} \) would improve $3.3\%$ and $4.6\%$ compared to Grounded-SAM~\cite{liu2023grounding}. If we further apply our proposed $L_{contra}$ to perform contrastive learning at frame level and video level, the box and segmentation score would improve to $74.4\%$ and $70.6\%$, which are $1.2\%$ and $0.8\%$ higher. Finally, if we directly take the ground-truth boxes to prompt SAM, the superior performance of $83.6\%$ in \( \mathcal{J} \)\&\( \mathcal{F} \) would be observed. This demonstrates that image segmentation could be mostly solved by SAM, and therefore how to generate proper prompts to instruct foundation segmentation models for referring segmentation tasks would now be of interest. From the above experiments, we confirm that our proposed loss functions would learn precise position prompts (box proposals) from the referring sentence and the input video, allowing efficient adaptation of foundation models for addressing RVOS.

\subsection{More Qualitative Comparisons}
For more qualitative comparisons, please refer to the video files in the supplementary materials or the following link: \url{https://drive.google.com/file/d/1MCF6jVqMBUnAbDMdZSTWt36L5HNClXLn/view?usp=sharing}.

% \section{More Implementation Details}
% We set the learning rate to $0.0001$ and train our framework for $12$ epochs. Following~\cite{liu2023grounding}, we set $\lambda_r$ and $\lambda_g$ as $5$ and $2$ respectively. As for $\lambda_f$ and $\lambda_v$, we use $0.01$ and $0.1$ on Ref-Youtube-VOS and $0.0001$ and $0.001$ on A2D Sentences, respectively. We implement our framework in PyTorch and train the model on $8$ NVIDIA V100 GPUs.

% \section{Rationale}
% \label{sec:rationale}
% % 
% Having the supplementary compiled together with the main paper means that:
% % 
% \begin{itemize}
% \item The supplementary can back-reference sections of the main paper, for example, we can refer to \cref{sec:intro};
% \item The main paper can forward reference sub-sections within the supplementary explicitly (e.g. referring to a particular experiment); 
% \item When submitted to arXiv, the supplementary will already included at the end of the paper.
% \end{itemize}
% % 
% To split the supplementary pages from the main paper, you can use \href{https://support.apple.com/en-ca/guide/preview/prvw11793/mac#:~:text=Delete%20a%20page%20from%20a,or%20choose%20Edit%20%3E%20Delete).}{Preview (on macOS)}, \href{https://www.adobe.com/acrobat/how-to/delete-pages-from-pdf.html#:~:text=Choose%20%E2%80%9CTools%E2%80%9D%20%3E%20%E2%80%9COrganize,or%20pages%20from%20the%20file.}{Adobe Acrobat} (on all OSs), as well as \href{https://superuser.com/questions/517986/is-it-possible-to-delete-some-pages-of-a-pdf-document}{command line tools}.
